# Supplementary material for: Target-Consistent Action Guidance via Semi-Unbalanced Optimal Transport for Drifting World Models
Source: arXiv:2611.24222 source file (2026-11-18)
Supplement: Supplementary file 1 [file X_suppl.tex]

%% =====================================================================
%% Supplementary material: Supp. A-G
%%   A Proofs (done) | B Experimental details (draft) | C Toy study of the target bias (text to write)
%%   D Unbalanced transport and relaxation patterns (draft) | E Additional results (partial)
%%   F Qualitative results (protocol done) | G Limitations (to do)
%% Cross-references: main.tex inputs this file after the bibliography and \appendix below starts the
%% lettered sections, so \ref{supp:...} in the main text resolves in the same document. If the supplement
%% is split into its own PDF for submission, use the xr package instead (\usepackage{xr} and
%% \externaldocument{<other aux file>} in each document). The label map is at the end of this file.
%% =====================================================================
\clearpage
\setcounter{page}{1}
\maketitlesupplementary


\appendix

\section{Proofs}
\label{sec:supp:proofs}\label{supp:proofs}

This section proves the propositions of the main paper.
We use the notation of the main paper.
At a single feature location, $d=y^+-o_t$ is the recorded motion, $m=\|d\|$, and $M=m^2+\delta$.

\subsection{Proof of Proposition 1 (residual push and overshoot)}
\label{supp:proof:p1}

\textit{Part (i).}
Let $q_\theta=\delta_{y^+}$, so the accentuated negatives are
\begin{equation*}
  \tilde q=(1-\gamma)\,\delta_{y^+}+\gamma\,\delta_{o_t}.
\end{equation*}
With a single positive, the attraction at $x=y^+$ is
\begin{equation*}
  V^+_p(y^+)=y^+-y^+=0.
\end{equation*}
The repulsion is the kernel-weighted mean of $y^--y^+$ over $\tilde q$.
Using $k(y^+,y^+)=1$ and $\kappa=k(y^+,o_t)$, its numerator is
\begin{equation*}
  (1-\gamma)\cdot 1\cdot(y^+-y^+)+\gamma\,\kappa\,(o_t-y^+)=-\gamma\kappa\,d,
\end{equation*}
and its denominator is
\begin{equation*}
  (1-\gamma)\cdot 1+\gamma\,\kappa.
\end{equation*}
Hence
\begin{align*}
  V^-_{\tilde q}(y^+)&=-\omega(y^+)\,d,\\
  V_{p,\tilde q}(y^+)&=V^+_p(y^+)-V^-_{\tilde q}(y^+)=\omega(y^+)\,d.
\end{align*}
For $\gamma>0$ and $\kappa>0$, the numerator $\gamma\kappa$ is positive and smaller than the denominator, so $\omega(y^+)\in(0,1)$.

\textit{Part (ii).}
Let $q_\theta=\delta_x$ with $x=o_t+t\,d$, so $x-o_t=t\,d$ and $y^+-x=(1-t)\,d$.
The negatives are $(1-\gamma)\,\delta_x+\gamma\,\delta_{o_t}$, and the same computation as in part (i) gives
\begin{equation*}
  V^-_{\tilde q}(x)=\frac{\gamma\kappa(x)\,(o_t-x)}{(1-\gamma)+\gamma\kappa(x)}=-\omega(x)\,t\,d.
\end{equation*}
The field is therefore a multiple of $d$,
\begin{equation*}
  V_{p,\tilde q}(x)=(1-t)\,d+\omega(x)\,t\,d=f(t)\,d,
  \qquad
  f(t)=1-t+\omega(x)\,t.
\end{equation*}
Since $k$ is radial, $\kappa(x)$ depends only on $\|x-o_t\|=t\|d\|$, so $f$ is continuous in $t$.
At $t=1$,
\begin{equation*}
  f(1)=\omega(y^+)>0.
\end{equation*}
As $t\to\infty$, $\kappa\to 0$, so $\omega\to 0$ and $f(t)=1-t(1-\omega)\to-\infty$.
By continuity, $f$ has a root $t^\star>1$, at which
\begin{equation*}
  1-t^\star+\omega(x^\star)\,t^\star=0
  \;\Longleftrightarrow\;
  t^\star=\frac{1}{1-\omega(x^\star)}.
\end{equation*}

\subsection{Proof of Proposition 2 (target bias of Wasserstein accentuation)}
\label{supp:proof:p2}

\textit{Part (i).}
Let $q=q'=\delta_x$.
The self coupling sends $x$ to itself, so $T_{q,q'}(x)=x$ and the base field is
\begin{equation*}
  V_0=y^+-T_{q,q'}(x)=y^+-x.
\end{equation*}
Adding the balanced accentuation term $A^{\mathrm{bal}}=(\alpha-1)d$ gives
\begin{equation*}
  V_0+A^{\mathrm{bal}}=y^+-x+(\alpha-1)\,d.
\end{equation*}
This vanishes if and only if
\begin{equation*}
  x=x^\star=y^++(\alpha-1)\,d,
\end{equation*}
and $x^\star-y^+=(\alpha-1)d\neq 0$ whenever $\alpha>1$ and $d\neq 0$.

\textit{Part (ii).}
Consider the unbalanced problem between two unit-mass Dirac measures $\delta_{y^+}$ and $\delta_{o_t}$.
Any plan has the form $\pi=m_\pi\,\delta_{(y^+,o_t)}$ with $m_\pi\geq 0$, so both marginals have mass $m_\pi$ and each of the three $\mathrm{KL}$ terms equals
\begin{equation*}
  \mathrm{KL}(m_\pi\delta\,\|\,\delta)=m_\pi\log m_\pi-m_\pi+1.
\end{equation*}
The objective is therefore
\begin{equation*}
  J(m_\pi)=\frac{m_\pi\|d\|^2}{2}+(2\lambda+\varepsilon)\big(m_\pi\log m_\pi-m_\pi+1\big).
\end{equation*}
Setting the derivative to zero,
\begin{align*}
  J'(m_\pi)&=\frac{\|d\|^2}{2}+(2\lambda+\varepsilon)\log m_\pi=0,\\
  m_\pi&=\exp\!\Big(-\frac{\|d\|^2}{2(2\lambda+\varepsilon)}\Big).
\end{align*}
This is the transported-mass ratio $s_{o_t}(y^+)$.
The same computation with zero cost (from $y^+$ to $y^+$) gives $s_{y^+}(y^+)=1$.
Substituting $x_i=y^+$ into the unbalanced accentuation term,
\begin{align*}
  A^{\mathrm{UW}}(y^+)
  &=(\alpha-1)\big[s_{y^+}(y^+)\,(y^+-y^+)-s_{o_t}(y^+)\,(o_t-y^+)\big]\\
  &=(\alpha-1)\,s_{o_t}(y^+)\,d,
\end{align*}
which is nonzero for $\alpha>1$ and $d\neq 0$.

\subsection{Proof of Proposition 3 (closed-form allocation)}
\label{supp:proof:p3}

With the source marginal fixed, the terms $-\Pi_{iv}+a_ib_v$ of the generalized $\mathrm{KL}$ sum to a constant, and the problem separates over rows.
For row $i$ we minimize
\begin{equation*}
  \sum_{v}\Pi_{iv}C_{iv}+\varepsilon_J\sum_{v}\Pi_{iv}\log\frac{\Pi_{iv}}{a_ib_v}
  \quad\text{s.t.}\quad \sum_v\Pi_{iv}=a_i,
\end{equation*}
whose solution is the softmax
\begin{equation*}
  \Pi_{iv}=a_i\,\frac{b_v\,e^{-C_{iv}/\varepsilon_J}}{\sum_{u}b_u\,e^{-C_{iu}/\varepsilon_J}}.
\end{equation*}
With $b=(\tfrac12,\tfrac12)$, the share sent to $o_t$ is
\begin{equation*}
  r_i=\frac{e^{-C_{i,o_t}/\varepsilon_J}}{e^{-C_{i,o_t}/\varepsilon_J}+e^{-C_{i,y^+}/\varepsilon_J}}
  =\sigma\!\Big(\frac{C_{i,y^+}-C_{i,o_t}}{\varepsilon_J}\Big).
\end{equation*}
Let $z=x_i-o_t$, so that $x_i-y^+=z-d$.
Then
\begin{equation*}
  \|z-d\|^2-\|z\|^2=m^2-2\langle z,d\rangle=m^2(1-2t_i),
\end{equation*}
with $t_i=\langle z,d\rangle/m^2$.
Dividing by $2M$,
\begin{equation*}
  C_{i,y^+}-C_{i,o_t}=\frac{m^2}{M}\Big(\frac12-t_i\Big),
\end{equation*}
and therefore
\begin{equation*}
  r_i=\sigma\!\Big(\frac{m^2}{\varepsilon_J M}\Big(\frac12-t_i\Big)\Big)
  =\sigma\!\Big(\frac{\tfrac12-t_i}{\varepsilon_d}\Big),
  \qquad
  \varepsilon_d=\frac{\varepsilon_J M}{m^2}.
\end{equation*}

\subsection{Proof of Proposition 4 (bias correction)}
\label{supp:proof:p4}

Let $q=q'=\delta_x$ with $x=o_t+t\,d+e$ and $e\perp d$.
As in part (i) of A.2, $T_{q,q'}(x)=x$, so
\begin{equation*}
  V_0=y^+-x=(1-t)\,d-e.
\end{equation*}
All predictions share the same progress $t$, so the gate uses $r(t)$.
With the uncentered and the centred term, the fields are
\begin{align*}
  V^{\mathrm{unc}}&=g(t)\,d-e, & g(t)&=(1-t)+\beta\,r(t),\\
  V^{\mathrm{MSA}}&=g_0(t)\,d-e, & g_0(t)&=(1-t)+\beta\big(r(t)-r^+\big).
\end{align*}
Since $e\perp d$ and $d\neq 0$, each field vanishes if and only if $e=0$ and its scalar factor is zero.
The share $r(t)$ is strictly decreasing in $t$, so $g$ and $g_0$ are strictly decreasing and each has at most one root.

\textit{Case (ii).} $g_0(1)=0+\beta(r^+-r^+)=0$, so the only zero is $t=1$, that is, $x=y^+$.

\textit{Case (i).} At $t=1$,
\begin{equation*}
  g(1)=\beta\,r^+>0.
\end{equation*}
At $t_1=1+\beta r^+>1$ we have $r(t_1)<r^+$, so
\begin{equation*}
  g(t_1)=-\beta\,r^++\beta\,r(t_1)<0.
\end{equation*}
The root $\tilde t$ therefore lies in $(1,t_1)$, and $g(\tilde t)=0$ gives
\begin{equation*}
  \tilde t-1=\beta\,r(\tilde t)\in\big(0,\beta\,r^+\big).
\end{equation*}

\subsection{Proof of Proposition 5 (residual control)}
\label{supp:proof:p5}

The derivative of the logistic sigmoid is at most $\tfrac14$, so
\begin{equation*}
  \Big|\frac{\mathrm{d}r}{\mathrm{d}t}\Big|\leq\frac{1}{4\varepsilon_d}
  \quad\Longrightarrow\quad
  |r_i-r^+|\leq\frac{|t_i-1|}{4\varepsilon_d}.
\end{equation*}
Since $x_i-o_t-d=x_i-y^+$,
\begin{equation*}
  t_i-1=\frac{\langle x_i-o_t-d,\,d\rangle}{m^2}=\frac{\langle x_i-y^+,\,d\rangle}{m^2},
\end{equation*}
and by Cauchy--Schwarz
\begin{equation*}
  |t_i-1|\leq\frac{\|x_i-y^+\|}{m}.
\end{equation*}
Combining,
\begin{align*}
  \|G\,d\|=m\,|G|
  &\leq\frac{m}{N_{\mathrm{neg}}}\sum_{i}|r_i-r^+|\\
  &\leq\frac{1}{4\varepsilon_d}\cdot\frac{1}{N_{\mathrm{neg}}}\sum_{i}\|x_i-y^+\|.
\end{align*}

%% =====================================================================
\section{Experimental details}
\label{supp:details}

\subsection{Data and latents}
\label{supp:data}
Robomimic Lift and Can use 270/30 training/validation demonstrations, and BridgeV2 has 53,192/6,872 training/validation episodes.
The model predicts 4 frames (1 on BridgeV2) from 4 history frames and their actions, and longer rollouts are autoregressive.
Actions are 2-D agent targets on Push-T and 7-D end-effector deltas on Robomimic and BridgeV2 (with gripper).
Push-T uses the GPC world-model data (8 shards of 500 episodes each).
Push-T frames ($96\times96$) and Robomimic frames ($84\times84$) are upsampled to $288\times288$ and encoded by the SD3 VAE into $16\times36\times36$ latents; BridgeV2 frames ($256\times256$) give $16\times32\times32$ latents.
Generated latents are decoded with the same VAE for all pixel metrics.

\subsection{Training and hyperparameters}
\label{supp:training}
Within a dataset, all five methods use the same number of steps, data, and noise seeds, with one training run each.
Tab.~1 uses the 100k-step Push-T checkpoints and Tab.~4 the 80k-step BridgeV2 checkpoints; the Robomimic step is \textbf{TODO} and identical for all methods.
On Push-T and Robomimic the global batch size is 4, the learning rate $1.25\times10^{-5}$, and $N_{\mathrm{neg}}=16$; on BridgeV2 they are 2, $2.5\times10^{-5}$, and 64.
All fields are computed on the SD3 latents; no method uses a pretrained feature encoder.
MSA uses $\beta=1$, $\varepsilon_J=0.25$, $\delta=0.05$, and $\chi=1$ on every dataset, was not tuned per dataset, and computes its gate per $4\times4$ latent patch.
The clip $\mathrm{RMS}(A)\le\chi\,\mathrm{RMS}(V_0)$ applies to the MSA term only; the accentuation of the baselines is not clipped.
% Values removed from Sec. 5.1 when it was shortened (to be placed here): AdamW, learning rate 1.25e-5,
% 500-step warm-up, beta=(0.9,0.95), weight decay 0.01, gradient clipping 2.0; EMA decay 0.999 (EMA weights
% evaluated); about 6.6M parameters; training steps on one RTX 5090 (XXk).
\TODO{remaining training values (Robomimic step, optimizer details above)}

\subsection{Baselines}
\label{supp:baselines}
W-Flow uses $\varepsilon=0.05$.
The accentuated baselines sample $\alpha\sim\log\mathcal{U}[1,4]$ with 10\% of the mass at $\alpha=1$.
The ``+ constant push'' row of Tab.~6 is the W-Flow + acc.\ model of Tab.~1; ``+ joint softmax'' is the MSA configuration (fixed weight 1, no $\alpha$ input) with floor subtraction and averaging turned off.
UW-Flow (Tab.~7) uses the penalty $\lambda=1$ (Eq.~(4)) in each of its transport problems.

\subsection{Action metrics}
\label{supp:metrics:action}
The reward is the GPC reward on Push-T, the cube height on Lift, and the negative distance of the can to its target bin on Can.
The same readout is used for all methods.
Each of the 200 start states has 16 proposals of horizon 8.
The 16 proposals per start state are the recorded action chunk and Gaussian random-walk perturbations of it.
$\tau$ is Kendall's $\tau_b$ between predicted and simulated rewards, averaged over start states and over three generator-noise seeds of the same trained model.
With $d$ and $\hat d$ the simulated and the seed-averaged predicted final object displacements, centered over the proposals of each start state, the slope is $\sum\langle\hat d,d\rangle/\sum\|d\|^2$ and the correlation is $\sum\langle\hat d,d\rangle/(\sum\|\hat d\|^2\sum\|d\|^2)^{1/2}$, pooled over start states; the signal ratio of Fig.~4 is $\mathrm{RMS}(\hat d)/\mathrm{RMS}(d)$.
Noise is the RMS over noise seeds of the predicted object position for a fixed start state and proposal.
The object pose is read by a keypoint probe on Push-T and a frozen ResNet-18 on Robomimic.
The outcome bias is the mean absolute difference between predicted and simulated rewards, in the units of the GPC reward; the tail share is the fraction of (start, proposal) pairs whose predicted block position has a standard deviation above 30~px across noise seeds.

\subsection{Motion metrics}
\label{supp:metrics:motion}
Moving and static regions are obtained from a dilated mask of the ground-truth frame difference.
Static drift is measured on static pixels over generated frames 9--60 of 64-frame autoregressive rollouts.
The onset delay is the signed difference, in frames, between the predicted and the real onset of object motion after contact (negative: early), where the object counts as moving once its displacement exceeds the threshold (1~px or 3~px on Push-T, 2~mm or 5~mm on Robomimic), and the late fraction is the fraction of rollouts with a late predicted onset.
EPE is the RAFT~\cite{teed2020raft} endpoint error between generated and real flow on pixels whose real flow exceeds 0.5~px.

\subsection{BridgeV2 protocol}
\label{supp:bridge}
The evaluation subset is every 14th validation episode (491 episodes).
Controllability uses one random 12-frame window per episode (489 episodes are long enough): 4 real frames and 8 generated frames, with the actions replaced by those of another random window under identical noise.
The motion probe uses 200 random validation windows and 16 one-step samples each; with $u$ the last context latent, $y$ the real next latent, $d=y-u$, and $\bar x$ the sample mean, progress is $t=\langle\bar x-u,d\rangle/\|d\|^2$ (also on the 25\% most-moving latent cells), the off-motion error is $\|(\bar x-u)-t\,d\|^2/\|d\|^2$, and the spread is the RMS of the per-dimension sample standard deviation.
Quality metrics use full validation episodes generated in 8-frame chunks that restart from real frames, with SSIM, PSNR, and LPIPS computed against the VAE reconstruction of the real frames, FID~\cite{heusel2017fid} over all generated and real frames, and FVD~\cite{unterthiner2018fvd} on the first 16 generated frames of each video.

\subsection{Full-episode rollouts}
\label{supp:fullep}
\TODO{full-episode protocol (Tab.~5)}

\subsection{GPC-Rank}
\label{supp:gpcrank}
Each plan ranks 50 proposals with the frozen reward predictor of GPC and executes 9 actions, for at most 300 steps; the score is the maximum coverage IoU of the episode.
Policy~1 is a GPC diffusion policy trained for 100 epochs and Policy~2 is the released GPC checkpoint.
The 50 evaluation episodes are the same for all world models, and planning time is measured on one RTX~5090.

\subsection{Compute}
\label{supp:compute}
\TODO{compute}

%% =====================================================================
\section{Toy study of the target bias}
\label{supp:toy}
% Status: all results in toy_experiment/; text to write.

\subsection{T-block setup}
\label{supp:toy:setup}
\TODO{T-block setup}

\subsection{Fixed point versus accentuation scale}
\label{supp:toy:alpha}
\TODO{fixed point vs $\alpha$}

\subsection{Small motions}
\label{supp:toy:small}
\TODO{small motions}

\subsection{Training dynamics in the sprite world (lag regime)}
\label{supp:toy:sprite}
\TODO{training dynamics (sprite world, lag regime)}

\subsection{Push versus progress}
\label{supp:toy:push}
\TODO{push vs progress}

%% =====================================================================
\section{Unbalanced transport and relaxation patterns}
\label{supp:uwflow}

\subsection{Mechanism: the spreading coefficient}
\label{supp:uwflow:mechanism}
One training step solves up to three transport problems from the generated samples $x$: to $y^+$ (attraction), to the second generated batch (the self term), and, with accentuation, to $o_t$.
UW-Flow relaxes both marginals of each with one penalty $\lambda=1$; MSA relaxes none of them, and its gate is a separate semi-relaxed problem whose source marginal is exact.
With a single positive, relaxing the attraction weights the pull of each sample by a transported mass $s_{qp}(x)\propto\exp\!\big(-\|x-y^+\|^2/(2(\lambda+\varepsilon))\big)$, so distant samples are pulled less; with $s_{qq'}$ and $s_{qu}$ the masses of the self term and of the transport to $o_t$, this adds the spreading term $(s_{qq'}-s_{qp})(x-T_{q,q'}(x))$, and a relaxed transport to $o_t$ adds the contraction $(\alpha-1)(s_{qp}-s_{qu})(o_t-x)$.
The net spreading coefficient is $c=(s_{qq'}-s_{qp})-(\alpha-1)(s_{qp}-s_{qu})$, the difference of two state-dependent terms that must cancel for the spread to be stable.
The balanced accentuation of Eq.~(12) shifts every sample equally and has no effect on the spread, and neither has the shared translation of MSA.

\subsection{Relaxation configurations}
\label{supp:uwflow:patterns}
On Push-T at 15k steps (one training seed, Kendall $\tau$ over three sampling seeds, noise in px), relaxing only some of the problems fails in one of two ways.
Relaxing the attraction while a repulsion stays balanced diverges (attraction and accentuation relaxed: $\tau$ $-0.008$, noise 58; attraction and self term relaxed: $\tau$ 0.007, noise 31), although the normalized training loss stays at 1.
Relaxing a repulsion while the attraction stays balanced under-disperses (accentuation only: $\tau$ 0.244, slope 0.204, noise 0.38; self term only: $\tau$ 0.268, noise 1.21).
Relaxing all three is stable only near $\lambda=1$, where $c\approx 0.089-1.05\times0.094\approx 0$ ($\lambda=0.3$: $\tau$ 0.258, noise 10.35; $\lambda=1$: $\tau$ 0.320, noise 3.67, the Tab.~7 entry; $\lambda=3$: $\tau$ 0.267, noise 2.93).
Without accentuation the spreading is unopposed, and UW-Flow has more than twice the noise of W-Flow (7.80 vs.\ 3.30).
\TODO{all 12 relaxation configurations}

\subsection{Long-schedule (40k) behaviour}
\label{supp:uwflow:long}
The transported masses at 40k steps were not logged, so the degradation of UW-Flow + acc.\ at 40k is consistent with, but not shown to be, the loss of this cancellation.
\TODO{40k behaviour}

%% =====================================================================
\section{Additional results}
\label{supp:results}

\subsection{Gate statistics}
\label{supp:gate}
In Fig.~4(a,b), $G$ and $\bar t$ are logged on training batches and averaged over moving patches and predictions; the band is their spread over the steps of a logging window.

\subsection{Projected-residual baseline}
\label{supp:projres}
% Status: linear-gate runs in progress (lambda = 0.42 / 0.7 / 1.0).
\TODO{projected-residual baseline}

\subsection{Separate gate components}
\label{supp:gate:separate}
Tab.~\ref{tab:supp_gate_sep} removes floor subtraction and shared translation one at a time from MSA, with all other settings as in Tab.~6.

\begin{table}[h]
\centering
\caption{\textbf{Separate gate components} on Push-T. \emph{w/o floor}: shared push $\beta\,\bar r\,d$ without subtracting $r^+$; \emph{w/o sharing}: per-prediction push $\beta\,(r_i-r^+)\,d$.}
\label{tab:supp_gate_sep}
\footnotesize
\setlength{\tabcolsep}{3pt}
\begin{tabular}{l ccccc}
\toprule
Variant & $\tau_3\uparrow$ & Slope$\uparrow$ & Noise$\downarrow$ & Bias$\downarrow$ & Mov.\ MSE$\downarrow$ \\
\midrule
MSA w/o floor & \TODO{} & \TODO{} & \TODO{} & \TODO{} & \TODO{} \\
MSA w/o sharing & \TODO{} & \TODO{} & \TODO{} & \TODO{} & \TODO{} \\
MSA (ours) & 0.712 & 0.746 & 1.55 & 0.462 & 0.1699 \\
\bottomrule
\end{tabular}
\end{table}

\subsection{Standard frame metrics}
\label{supp:frame}
\TODO{standard frame metrics}

\subsection{Full-episode results per segment}
\label{supp:fullep:segment}
\TODO{full-episode per segment}

\subsection{Accentuation scale sweep}
\label{sec:supp:alpha}\label{supp:alpha}% kept from the previous supplement (was its own section)

\begin{table}[t]
\centering
\caption{\textbf{Accentuation scale sweep.} Results for each accentuated baseline and accentuation scale $\alpha$, and for MSA.}
\label{tab:supp_alpha}
\footnotesize
\setlength{\tabcolsep}{3pt}
\begin{tabular}{l c cccccc}
\toprule
Method & $\alpha$ & $\tau\uparrow$ & Slope$\uparrow$ & Noise$\downarrow$ & Bias$\downarrow$ & Mov.\ MSE$\downarrow$ & EPE$\downarrow$ \\
\midrule
Kernel + acc. & 1 & 0 & 0 & 0 & 0 & 0 & 0 \\
 & 1.5 & 0 & 0 & 0 & 0 & 0 & 0 \\
 & 2.5 & 0 & 0 & 0 & 0 & 0 & 0 \\
 & 4 & 0 & 0 & 0 & 0 & 0 & 0 \\
\midrule
W-Flow + acc. & 1 & 0 & 0 & 0 & 0 & 0 & 0 \\
 & 1.5 & 0 & 0 & 0 & 0 & 0 & 0 \\
 & 2.5 & 0 & 0 & 0 & 0 & 0 & 0 \\
 & 4 & 0 & 0 & 0 & 0 & 0 & 0 \\
\midrule
MSA (ours) & -- & 0 & 0 & 0 & 0 & 0 & 0 \\
\bottomrule
\end{tabular}
\end{table}

%% =====================================================================
\section{Qualitative results}
\label{supp:qual}

\subsection{Case-selection protocol}
\label{supp:qual:selection}
In Fig.~3 all models use the same context, recorded actions, and noise seed.
The BridgeV2 window was chosen by a search over 2,280 validation windows for clear, localized motion and was kept only if MSA was the closest to the ground truth on at least two of three noise seeds; the final choice was made by a judge who saw unlabeled, shuffled method columns.
% Full protocol: CASE_SELECTION_STRATEGY.md.

\subsection{Additional rollouts}
\label{supp:qual:more}
\TODO{additional rollouts}

%% =====================================================================
\section{Limitations}
\label{supp:limitations}
\TODO{limitations}

%% =====================================================================
%% Label map: generic "supplement" mentions in the main text -> supplement labels
%%   Sec. 4 (Props. 1-5): proofs -> supp:proof:p1 ... supp:proof:p5
%%   Sec. 5.1: latent-space kernel baselines -> supp:baselines; hyperparameters -> supp:training;
%%             metric definitions -> supp:metrics:action, supp:metrics:motion
%%   Sec. 5.3: BridgeV2 -> supp:bridge
%%   Sec. 5.4: GPC-Rank -> supp:gpcrank
%%   Sec. 5.5 / Fig. 1 / Tab. 3 (toy): toy -> supp:toy; lag regime -> supp:toy:sprite
%%   Sec. 5.6: full-episode -> supp:fullep
%%   Sec. 5.8: gate curves -> supp:gate
%%   Sec. 5.9: "the two nearly cancel (supplement)" -> supp:uwflow:mechanism, supp:uwflow:patterns
%%   Fig. 3 (qualitative): BridgeV2 case -> supp:qual:selection
%% =====================================================================
